# Supplementary material for: Disentangling Decentralized Finance (DeFi) Compositions
Source: arXiv:2111.11933 source file (2022-09-30)
Supplement: Supplementary file 1 [file supplemental.tex]

% !TeX root = ../main.tex

\section{Supplemental Material}
